# Supplementary material for: OCAtari: Object-Centric Atari 2600 Reinforcement Learning Environments
Source: arXiv:2306.08649 source file (2024-02-27)
Supplement: Supplementary file 1 [file supplementary.tex]

% Supplementary material: To improve readability, you must use a single-column format for the supplementary material.

\onecolumn
\begin{center}
\textbf{\large Supplemental Materials}
\end{center}
%\addcontentsline{toc}{section}{Appendix}
\setcounter{section}{0}

\section{Per Game evaluation}
\subsection*{Space Invaders:}
bullet in space invaders is something that is apparently random in its shown size and in its blinking. (random size could be seen from vision mode) so the size am giving is general so that its symbol is mostly (average) included in the rectangle, does this make sense? are size and blinking what you meant by detecting bullets more precisely?
by observing the ram, no value for a bullet being visible in the current moment could be determined(I tried it by excluding by observing and testing (not) changing values with (not) changing visibility in rgb . When it is invisible (while moving) it still moving but blinking. I did some small changes/improvements to not detect an invisible one out of the range of the game space and a change to detect it as vision when it is on the borders of ground. (rectangle gets smaller so its a detection like the one in vision).
\\
\\
(empty columns in) function make\_bitmap has been tested through setting same (and different) distributions of aliens to all lines(columns):
\begin{verbatim}
    (for i in range(6):
        )env._env.unwrapped.ale.setRAM(18 (+ i), 6)
\end{verbatim}

\subsection*{Seaquest}
Enemies and Submarines move slightly up and down all the time. In revised mode the y-Position is set to a constant in the middle of the upper and lower position of the enemies. But that lowers the IOU Score for enemies and submarines.\\
The player IOU is not perfect because in vision mode the player is sometimes not detected for example when he gets hit the color changes to white or when the surface water cuts off the top part of the Player.\\
Enemy and player missile are also not perfect in vision mode which lowers the IOU score. For example if the player shoots at the surface, the player missile is behind the water surface and thus not detected in vision mode but in revised mode the missile gets rightfully detected.

\subsection*{Tennis}
Player and enemy IOU are not perfect because their width changes depending on if they are facing to the left or to the right with the racket. Also during the animation of hitting the ball their model is slightly wider.\\
Ball and BallShadow IOU are not perfect because both are very small objects and in revised their y-Position is sometimes a little bit over them or underneath them. 

\subsection*{Carnival}
Player Missile is very bad because no RAM value was found that saves the x-Position of the missile. That let to the assumption that the missiles x-Position is based on the x-Position of the player. However no perfect offset was found because the missile is only 1 Pixel wide. Also the height of the missile changes randomly. Sometimes it is just a little dot and sometimes its height is up to 20. For those reasons the width of the missile is set much wider so that in most cases the missile is somewhere in the wider box which detects the PlayerMissile.

\subsection*{Breakout}
Works fine.

\subsection*{Bowling}
Works fine.

\subsection*{Berzerk}
Player and Enemy missiles IOU gets worse because for a random amount of time the missile is still shown when it hits a wall. The RAM value for the x-Position of the missiles reset to 0 but they are rendered as if they are stuck in the wall at the previous position.

\subsection*{Kangaroo}
The player IOU is bad due to the jumping animation of the Kangaroo. When performing a jump the sprite size gets smaller when reaching the peak hight of a jump. It is hard to pin down the exact moment to switch the bounding box size.
The child IOU somtimes gets messed up when it is standing on the right, also the y position is a fixed value in the revised mode, therefor jumping will not be detected.
The projectile falling from top gets messed up since it has the same colors as the floors, ladders and walls. This leads to the vision mode not detecting it properly and lowering the IOU.
The enemys position on screen sometimes do not match their y value in the RAM. Occasionly the enemys will step out of the wall onto the floor and their x positions will sometimes differ from the given value in the RAM (Only seen in the reports files, dont know how to reproduce the Error). 
The enemy projectile has the same color as the enemy, which results in it beeing detected as part an enemyin vision mode when close by the thrower. Also the position in the RAM does not represent the projectile position perfectly, making the projectile stick out of either the left or right side depending on the viewed frame (its random).
The fruit IOU gets messed up by the game tending to flicker during gameplay. This affects the fruits the most.

\subsection*{MsPacman}
Player IOU is bad since the sprite sometimes lags behind the RAM value. The amount of lag and the timing seems to be random.
Enemy IOU suffers from the high amount of flickering in the game especially when two or more ghosts overlap.
Just as the player the fruits visual rendering does not always match the RAM value making it tank some of its IOU.

\subsection*{Assault}
PlayerMissileHorizontal is not perfect, because like in other games the x-Position of the missile is not stored in the RAM. That is why the position of the player is used when the missile appears and every frame an offset is added, however in the game the offset is not constant.\\
EnemyMissile faces the same problem. The RAM also does not save the x-Position for the enemy missile, so the position of the enemy is used when the missile is fired. However this does not get the perfect x-Position for the missile.
